# Supplementary material for: A Robotic Model of Hippocampal Reverse Replay for Reinforcement Learning
Source: arXiv:2102.11914 source file (2021-02-23)
Supplement: Supplementary file 1 [file supplementary_material.tex]

\section*{Supplementary Material}
\subsection{Algorithmic Implementation of the Network}

\noindent\fbox{%
    \parbox{\textwidth}{%
        \textbf{Box 1: Algorithmic Implementation}
        
        \begin{enumerate}
            \item Initialisation: 
            \begin{itemize}
                \item MiRo is placed into a random start location.
                \item All place cell variables set to steady state conditions for zero place cell input.
                \item All action cell values set to zero.
                \item Weights $w_{ij}^{PC\text{-}AC}$ randomised and normalised:\\ $w_{ij}^{PC\text{-}AC} \leftarrow \frac{w_{ij}^{PC\text{-}AC}}{\sum_i w_{ij}^{PC\text{-}AC}}$.
            \end{itemize}
            \item Determine MiRo's movement and reward values:
            \begin{itemize}
                \item If found\_goal:
                \begin{itemize}
                    \item $R = 1$; $\lambda = 1$; MiRo\_movement = stalled.
                    \item Update weights according to Equation 28.
                    \item If this experiment includes replays: 
                    \begin{itemize}
                        \item After 1s and For 0.1s initiate place cell replays by setting: $I^{place}_j = I^{p}_{max} \text{exp}\left[- \frac{(x_{MiRo}^c - x_j^c)^2 + (y_{MiRo}^c - y_j^c)^2}{2d^2} \right]$. 
                        \item Update weights and eligibility traces according to Equations. \ref{eqtn:learning_rule_replay} and \ref{eqtn:eligibility_trace_replay}.
                    \end{itemize}
                    \item After 2s: $R=0$; $\lambda = 0$; MiRo\_movement = move\_to\_random\_location.
                \end{itemize}
                \item Else If detected\_wall:
                \begin{itemize}
                    \item For 0.5s: $R = -1$.
                    \item MiRo\_movement = wall\_avoidance\_procedure.
                    \item Update weights according to Equation 28.
                \end{itemize}
                \item Else:
                \begin{itemize}
                    \item $R = 0$.
                    \item If 0.5s has passed since last action:
                    \begin{itemize}
                        \item If $M_{PC\_proposal} > 1$: $y_i \sim \mathcal{N}\left( \tilde{y}_i, \sigma^2 \right) \; \forall \, i$
                        \item Else: $y_i = y_i^{random\_walk} \; \forall \, i$.
                        \item Compute $\theta_{target}$ from $y_i$ and set MiRo\_movement to move towards this heading with constant forward velocity.
                    \end{itemize}
                \end{itemize}
            \end{itemize}
        \end{enumerate}
    }%
}

\newpage

\noindent\fbox{%
    \parbox{\textwidth}{%
        \textbf{Box 1: Algorithmic Implementation -- Continued}
        
        \begin{enumerate}
        \setcounter{enumi}{2}
            \item Update network variables:
            \begin{itemize}
                \item Update place cells based on MiRo's position in the environment.
                \item Use place cell values and action cell values to update eligibility traces according to Equation \ref{eqtn:eligibility_trace}.
            \end{itemize}
            \item Return to Step 2 and repeat.
        \end{enumerate}
    }%
}

\newpage
\subsection*{Effects of Removing Global Inhibition on Reverse Replays}
Shown here is the effect that removing global inhibition for the place cell network, as found in \cite{whelan2020fast}, does not impact the ability of the network to produce reverse replays.

\setcounter{figure}{0}
\makeatletter 
\renewcommand{\thefigure}{S\@arabic\c@figure}
\makeatother
\begin{figure}[h!]
    \centering
    \includegraphics[width=0.8\textwidth]{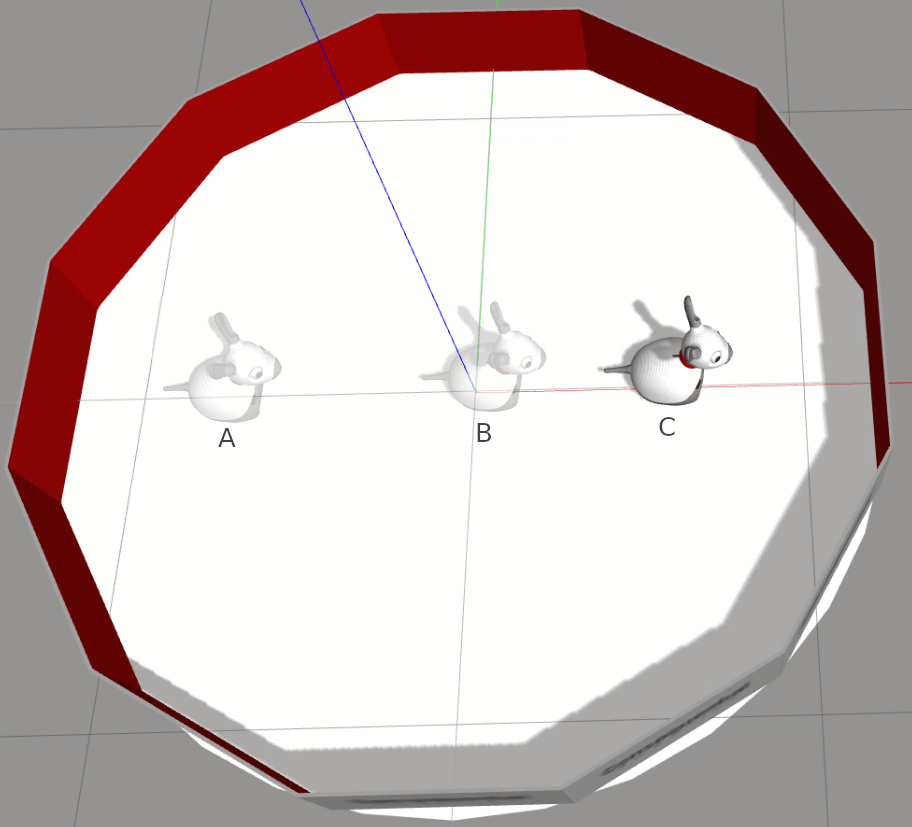}
    \caption[Example of a straight trajectory by MiRo]{The example trajectory used to show there is no effect on reverse replays with or without the inhibitory term. MiRo begins in position A, passes through position B and ends in position C.}
    \label{fig:straight_line}
\end{figure}
\begin{figure}[h!]
    \centering
    \includegraphics[width=\textwidth]{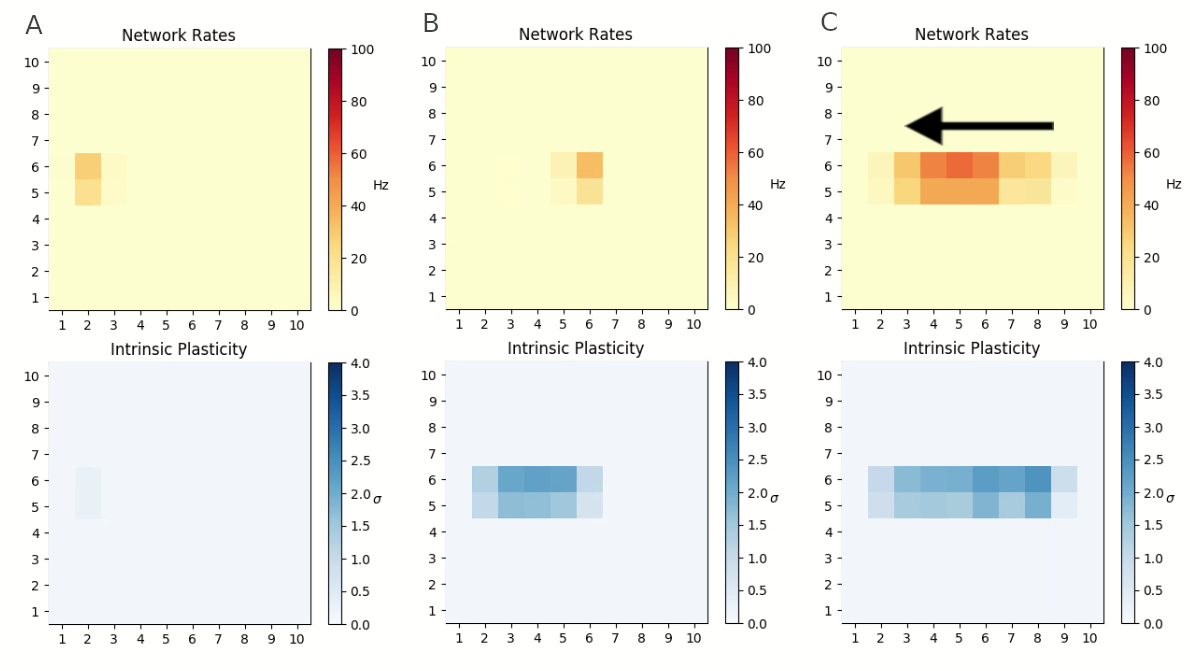}
    \caption[Plots of place cell rates and intrinsic plasticities for the straight line trajectory]{Plots of the place cell rates and intrinsic plasticities as MiRo passes through the points marked A, B and C in Figure \ref{fig:straight_line}. Note that the activity in C is that of the reverse replay event, with the arrow indicating the temporal ordering of firing of the cells.}
    \label{fig:straight_line_plots}
\end{figure}
\begin{figure}[h!]
    \centering
    \includegraphics{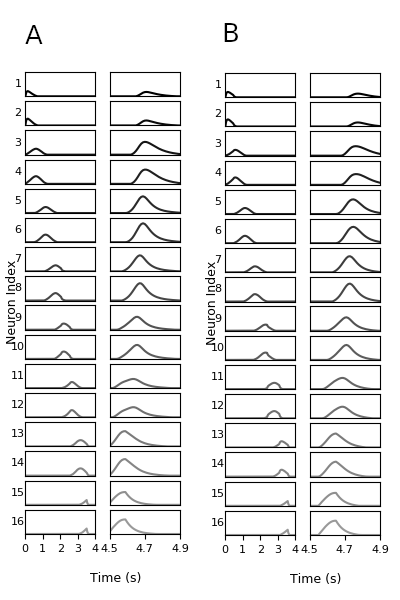}
    \caption[Line plots of the place cell rates for the straight line trajectory]{Line plots of the temporal ordering for the place cells that fired during the trajectory in Figure \ref{fig:straight_line}. Plot (A) gives the rates without inhibition, whilst plot (B) is with inhibition. Left hand side plots in each is the activity during the trajectory, whilst the right hand side plots are during a reverse replay. In both cases reverse replays of the trajectory are produced.}
    \label{fig:straight_line_line_plots}
\end{figure}

\clearpage
\subsection*{Further Simulation Results}
The experiments with and without replays were run over a wide range of parameter values for $\uptau_e$ and $\eta$. Experiments were performed across values of $\uptau=0.04s, 0.2s, 1s, 5s$ and $\eta = 0.001, 0.01, 0.1, 1$. Plots of the average times to reward retrieval, averaged over 40 independent experiments, for all parameters are shown over the four figures given here. As before, solid lines indicate the averages whilst shaded regions show one standard deviation.

What is most noticeable across these results is that replays offer the most significant advantage when the eligibility trace time constant, $\uptau_e$, is small. As this time constant gets larger, replays offer little to no advantage over non-replays. However, if the eligibility trace time constant grows too large, performance worsens anyway in both replay and non-replay cases.

\begin{figure}[h!]
    \centering
    \includegraphics[width=0.85\textwidth]{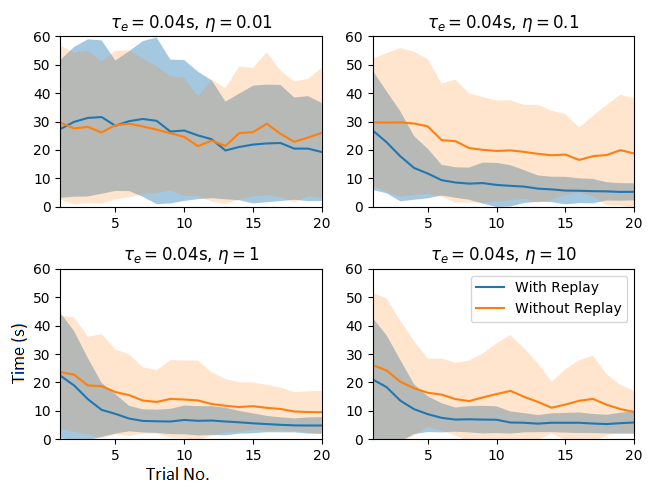}
    \caption{Full results for $\uptau_e = 0.04s$}
    \label{fig:my_label}
\end{figure}

\begin{figure}[h!]
    \centering
    \includegraphics[width=0.85\textwidth]{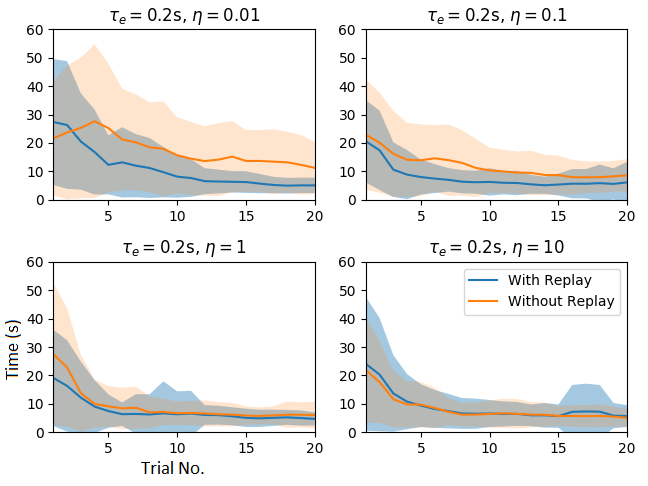}
    \caption{Full results for $\uptau_e = 0.2s$}
    \label{fig:tau_e = 0.04s}
\end{figure}

\begin{figure}[h!]
    \centering
    \includegraphics[width=0.85\textwidth]{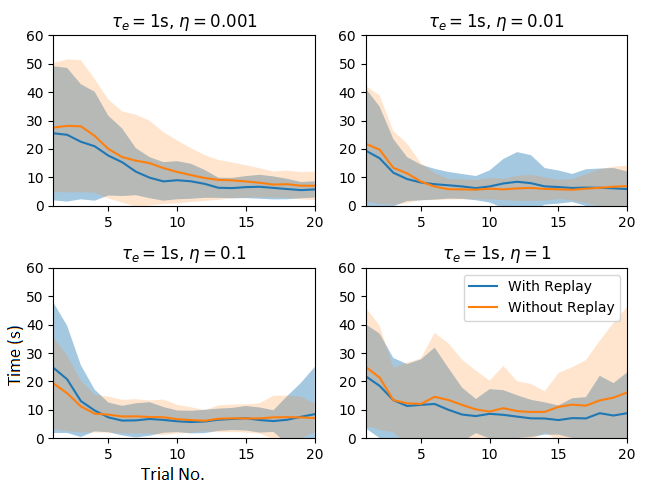}
    \caption{Full results for $\uptau_e = 1s$}
    \label{fig:tau_e = 1s}
\end{figure}

\begin{figure}[h!]
    \centering
    \includegraphics[width=0.85\textwidth]{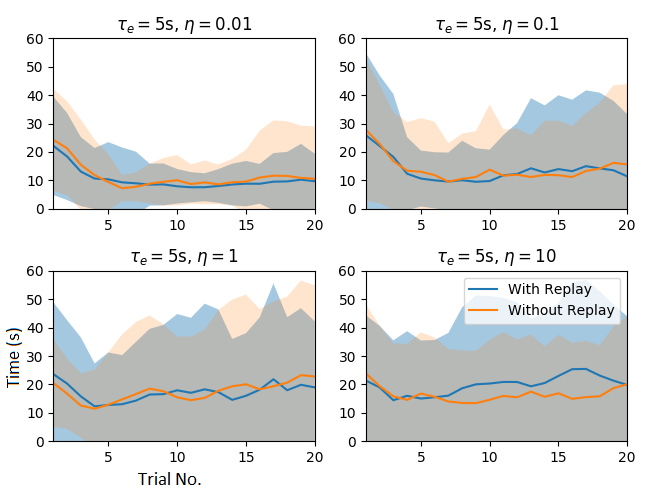}
    \caption{Full results for $\uptau_e = 5s$}
    \label{fig:tau_e = 5s}
\end{figure}

\begin{figure}[h!]
    \centering
    \includegraphics[width=0.85\textwidth]{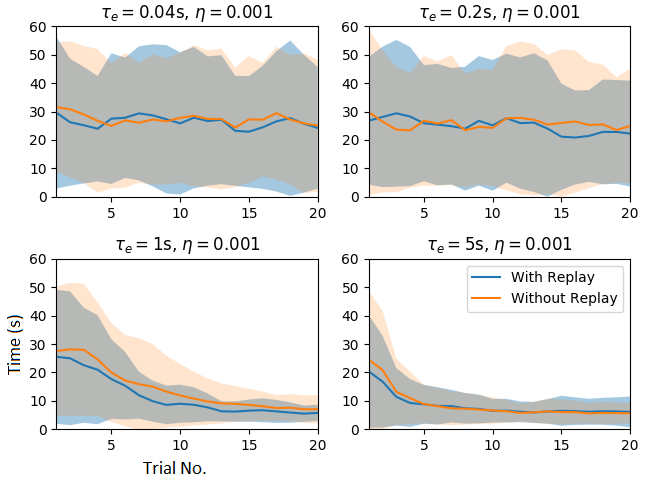}
    \caption{Full results for $\eta = 0.001$}
    \label{fig:eta = 0.001}
\end{figure}

\clearpage
\subsection{Best Case Comparison Table of Results}
The table of results for the best case comparison shown in Figure \ref{fig:comparing_best_cases} is given here. The p-value and z-scores for each trial is given, which indicates divergence of similarity past trial 19. Significant differences, where $p<0.05$, are highlighted in bold.

\begin{center}
 \begin{tabular}{||c c c||} 
 \hline
 Trial No. & p-value & z-score \\ [0.5ex] 
 \hline\hline
 15 & .121 & -1.1656 \\ 
 \hline
 16 & .40129 & -0.2493 \\
 \hline
 17 & .32997 & -0.4401 \\
 \hline
 18 & .2177 & -0.7805 \\
 \hline
 \textbf{19} & \textbf{.0099} & \textbf{-2.328} \\
 \hline
 20 & .47608 & -0.0567 \\
 \hline
 \textbf{21} & \textbf{.03074} & \textbf{-1.8687} \\
 \hline
 \textbf{22} & \textbf{.0057} & \textbf{-2.5306} \\
 \hline
 \textbf{23} & \textbf{.00776} & \textbf{-2.4223} \\
 \hline
 \textbf{24} & \textbf{.04272} & \textbf{-1.7174} \\
 \hline
 \textbf{25} & \textbf{.01539} & \textbf{-2.164} \\
 \hline
 26 & .15625 & -1.0109 \\
 \hline
 \textbf{27} & \textbf{.0057} & \textbf{-2.5254} \\
 \hline
 \textbf{28} & \textbf{.015} & \textbf{-2.1679} \\
 \hline
 29 & .18141 & -0.9145 \\
 \hline
 30 & .05592 & -1.5881 \\ [1ex] 
 \hline
\end{tabular}
\end{center}
